# Supplementary material for: A substandard candle: the low-$\nu$ method at few-GeV neutrino energies
Source: arXiv:2203.11821 ancillary file (2023-03-06)
Supplement: Supplementary file 1 [file supplementary_material.pdf]

# Supplementary Material: A substandard candle: the low-$\nu$ method at few-GeV neutrino energies

## Energy-transfer Variable Definitions

- $q_0 = E_\nu - E_\ell$ — The true energy transfer from the interacting lepton system, experimentally unobservable.
- $E_{\mathrm{had}}^{\mathrm{true}} = \left(\sum_{i=n,p} E_{\mathrm{kin}}^i\right) + \left(\sum_{i=\pi^\pm,\pi^0,\gamma} E_{\mathrm{total}}^i\right)$ — the true hadronic energy is defined as the sum of the kinetic energies of the protons and neutrons, and the total energy of all pions and photons. Other hadrons can be neglected at the energy transfers of interest. This variable is what could be seen by a "perfect" detector capable of measuring and identifying all outgoing particles without threshold or uncertainty, including neutrons.
- $E_{\mathrm{had}}^{\mathrm{reco}} = \left(\sum_{i=p} E_{\mathrm{kin}}^i\right) + \left(\sum_{i=\pi^\pm,\pi^0,\gamma} E_{\mathrm{total}}^i\right)$ — the reconstructed hadronic energy is the same as $E_{\mathrm{had}}^{\mathrm{true}}$, but without including neutrons. Experiments typically recover some fraction of the neutron energy, but reliably measuring the total neutron energy event-by-event is extremely challenging.
- $E_{\mathrm{avail}} = \left(\sum_{i=\pi^\pm,p} E_{\mathrm{kin}}^i\right) + \left(\sum_{i=\pi^0,\gamma} E_{\mathrm{total}}^i\right)$ — the available, or recoil, energy is the calorimetric sum of the outgoing hadronic state. Given the low energy transfers of interest, it is a proxy for the energy seen in a detector with a high tracking threshold, where individual charged-pions are not identified, and no neutron energy is measured.

## Sample Generation

For each model, $1 \times 10^8$ neutrino interactions were simulated according to a uniform neutrino energy spectrum between 0–15 GeV. It is worth noting that while the neutrino *flux* energy spectrum is uniform during generation, because the cross section increases as a function of neutrino energy and so the shape of the generated event rate in neutrino energy will follow the shape of the modelled cross section. More details of the generator configurations are available upon request.

## Table of contents

For each energy-transfer proxy variable, for muon neutrinos and antineutrinos, and for hydrocarbon and water targets, the predicted cross-section from each model is shown over a range of cut values on the proxy variable of interest. For easy access to specific sets of figures, the table below links to the relevant page in the rest of the document.


| | $\nu_\mu$ | $\bar{\nu}_\mu$ |
|---|---|---|
| $q_0$ | $C_nH_n$ $^{40}Ar$ | $C_nH_n$ $^{40}Ar$ |
| $E_{\mathrm{had}}^{\mathrm{true}}$ | $C_nH_n$ $^{40}Ar$ | $C_nH_n$ $^{40}Ar$ |
| $E_{\mathrm{had}}^{\mathrm{reco}}$ | $C_nH_n$ $^{40}Ar$ | $C_nH_n$ $^{40}Ar$ |
| $E_{\mathrm{avail}}$ | $C_nH_n$ $^{40}Ar$ | $C_nH_n$ $^{40}Ar$ |

# $\nu_\mu$ Interacting with a $C_nH_n$ Target

## $\nu_\mu$ Interacting with a $C_nH_n$ Target: Cutting on $q_0$

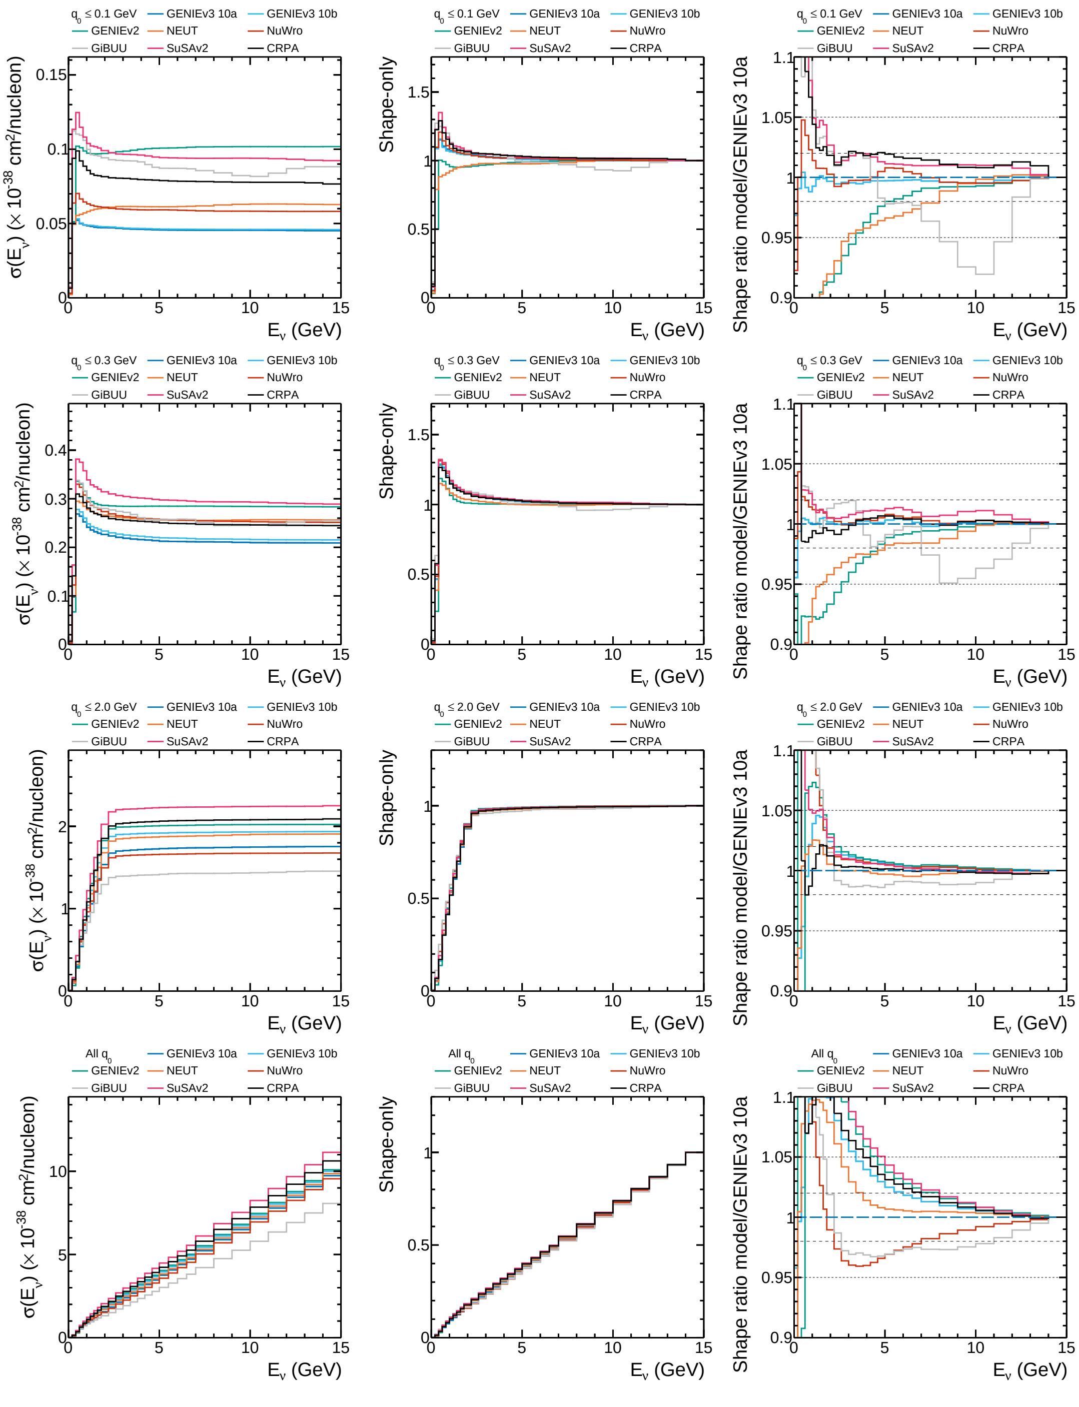


Figure 1: A comparison of the various generator predictions for different $q_0$ cuts. The absolute $\nu_\mu$ on $C_nH_n$ cross section per nucleon (left column), a shape-only comparison where each prediction is normalized to give the same prediction for the 14–15 GeV bin (center column), and the variation of each shape-only prediction relative to a GENIEv3 10a reference prediction (right column). The four rows show the effect of increasing the $q_0$ cut 0.1 GeV, 0.3 GeV, 2.0 GeV, or having no cut, when attempting to isolate a low-$\nu$ sample.

## $\nu_\mu$ Interacting with a $C_nH_n$ Target: Cutting on $E_{\rm had}^{\rm true}$

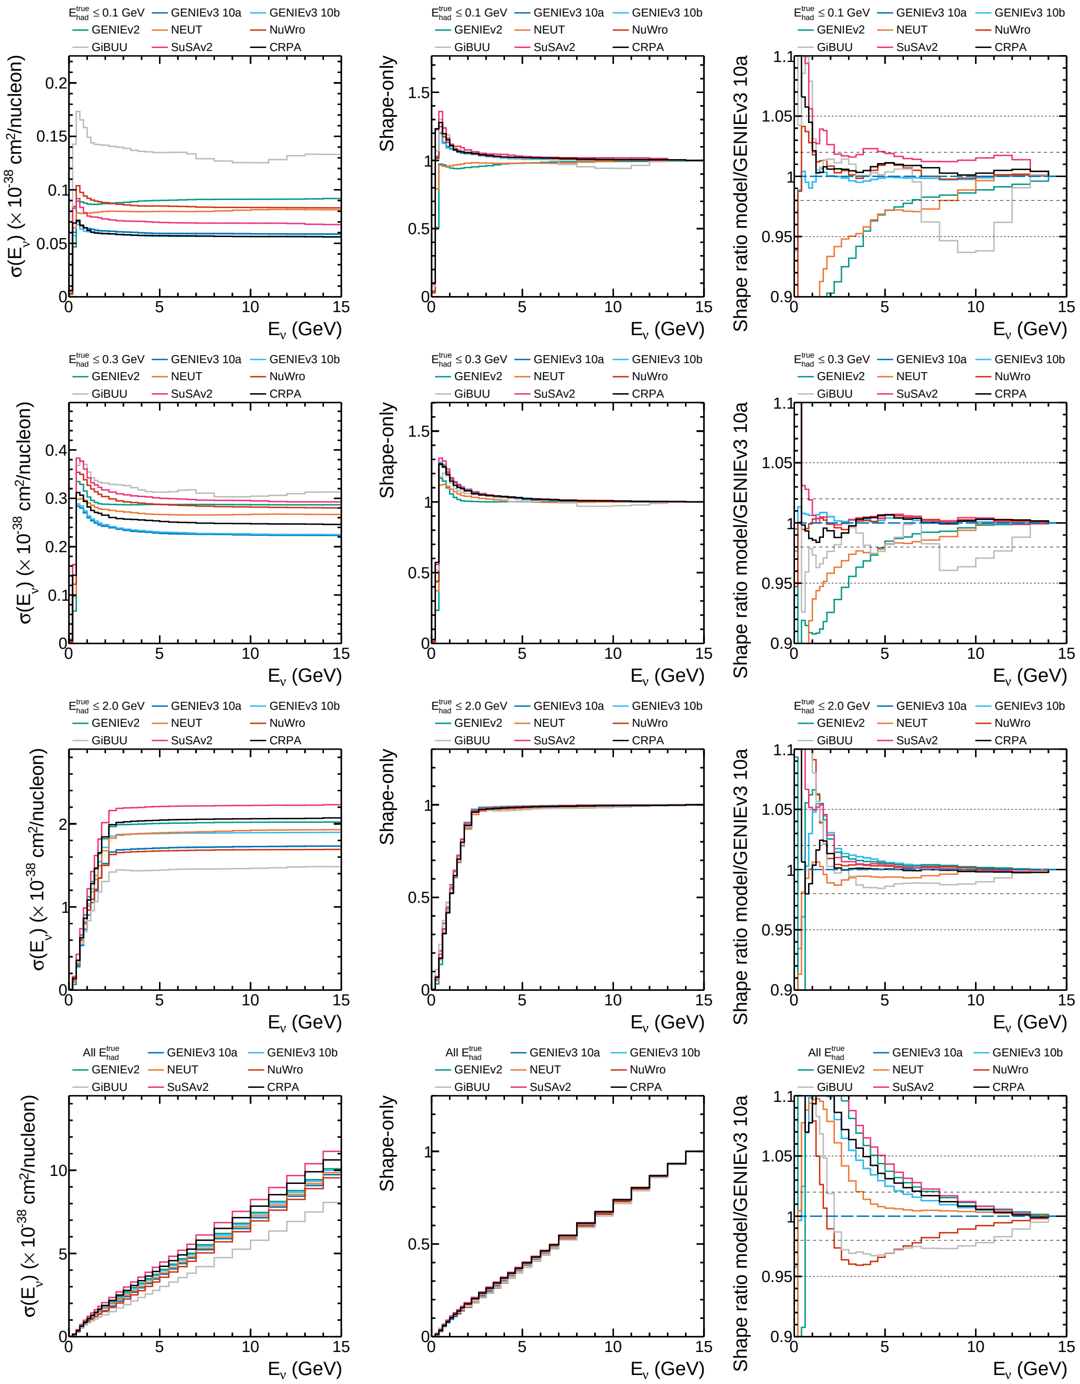


Figure 2: A comparison of the various generator predictions for different $E_{\rm had}^{\rm true}$ cuts. The absolute $\nu_\mu$ on $C_nH_n$ cross section per nucleon (left column), a shape-only comparison where each prediction is normalized to give the same prediction for the 14–15 GeV bin (center column), and the variation of each shape-only prediction relative to a GENIEv3 10a reference prediction (right column). The four rows show the effect of increasing the $E_{\rm had}^{\rm true}$ cut 0.1 GeV, 0.3 GeV, 2.0 GeV, or having no cut, when attempting to isolate a low-$\nu$ sample.

## $\nu_\mu$ Interacting with a $C_nH_n$ Target: Cutting on $E_{\mathrm{had}}^{\mathrm{reco}}$

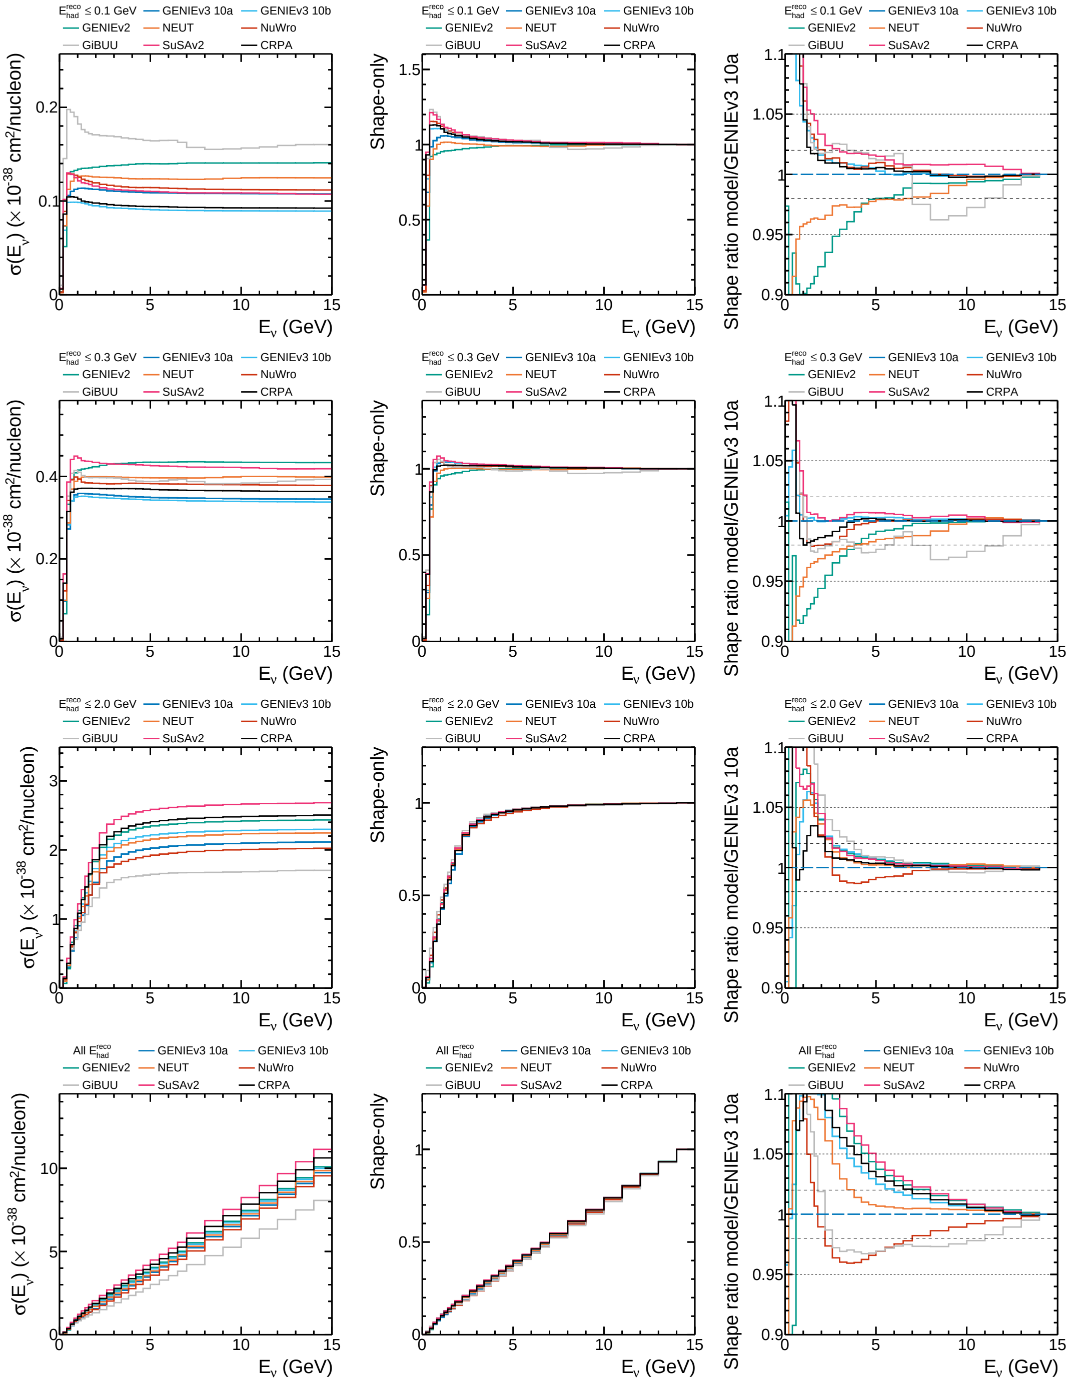


Figure 3: A comparison of the various generator predictions for different $E_{\mathrm{had}}^{\mathrm{reco}}$ cuts. The absolute $\nu_\mu$ on $C_nH_n$ cross section per nucleon (left column), a shape-only comparison where each prediction is normalized to give the same prediction for the 14–15 GeV bin (center column), and the variation of each shape-only prediction relative to a GENIEv3 10a reference prediction (right column). The four rows show the effect of increasing the $E_{\mathrm{had}}^{\mathrm{reco}}$ cut 0.1 GeV, 0.3 GeV, 2.0 GeV, or having no cut, when attempting to isolate a low-$\nu$ sample.

## $\nu_\mu$ Interacting with a $C_nH_n$ Target: Cutting on $E_{\text{avail}}$

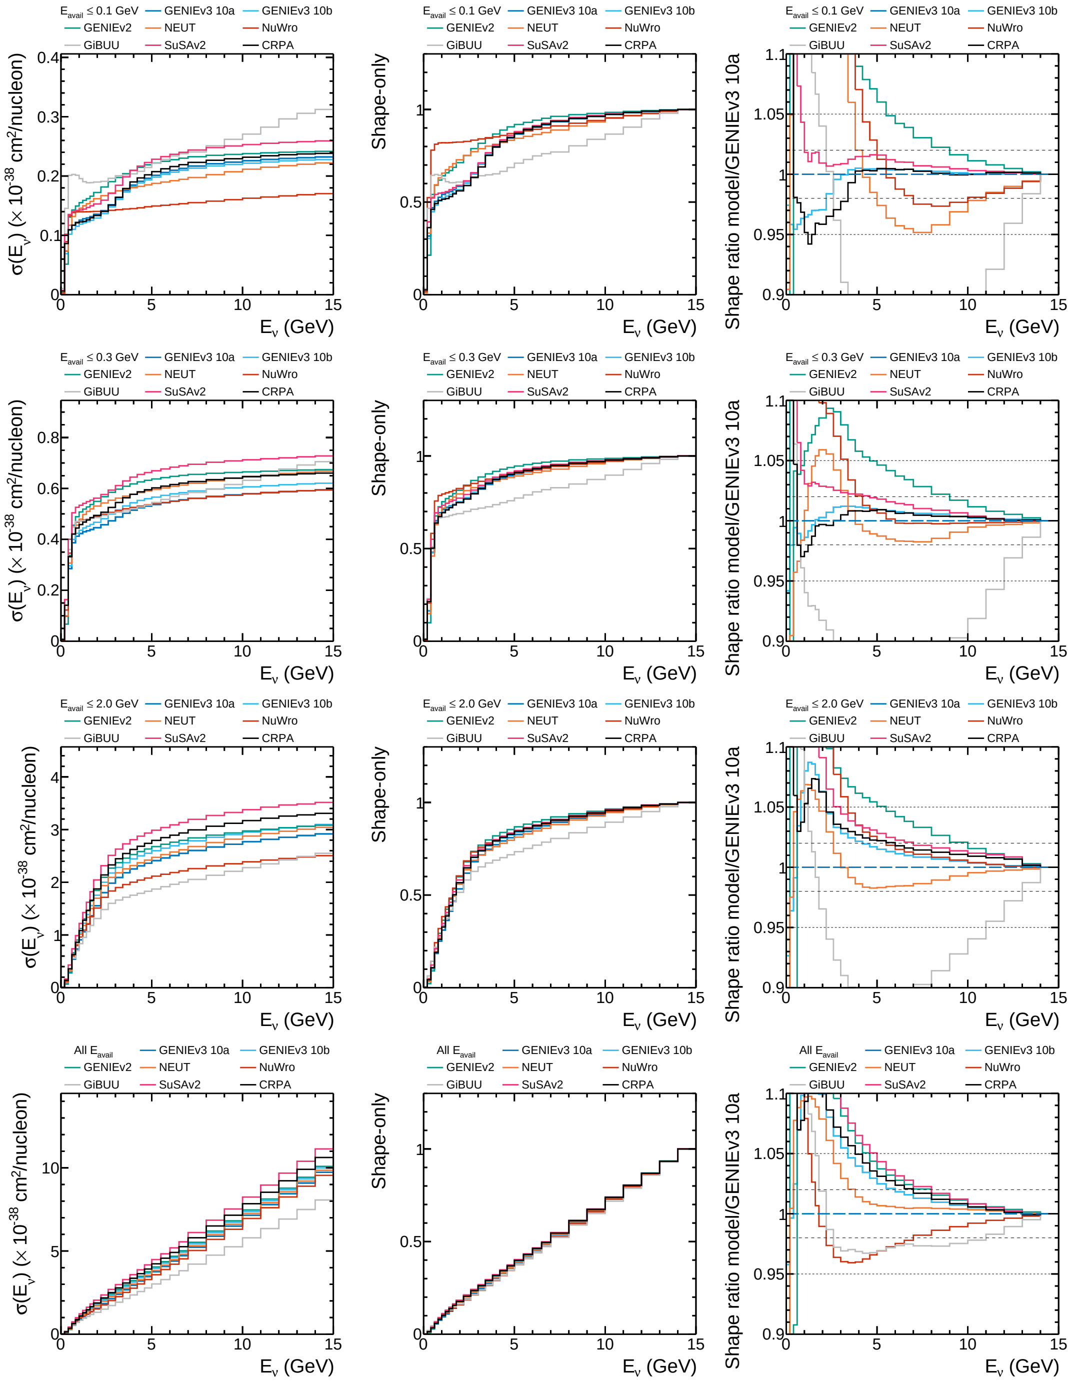


Figure 4: A comparison of the various generator predictions for different $E_{\text{avail}}$ cuts. The absolute $\nu_\mu$ on $C_nH_n$ cross section per nucleon (left column), a shape-only comparison where each prediction is normalized to give the same prediction for the 14–15 GeV bin (center column), and the variation of each shape-only prediction relative to a GENIEv3 10a reference prediction (right column). The four rows show the effect of increasing the $E_{\text{avail}}$ cut 0.1 GeV, 0.3 GeV, 2.0 GeV, or having no cut, when attempting to isolate a low-$\nu$ sample.

# $\bar{\nu}_\mu$ Interacting with a $C_nH_n$ Target

## $\bar{\nu}_\mu$ Interacting with a $C_nH_n$ Target: Cutting on $q_0$

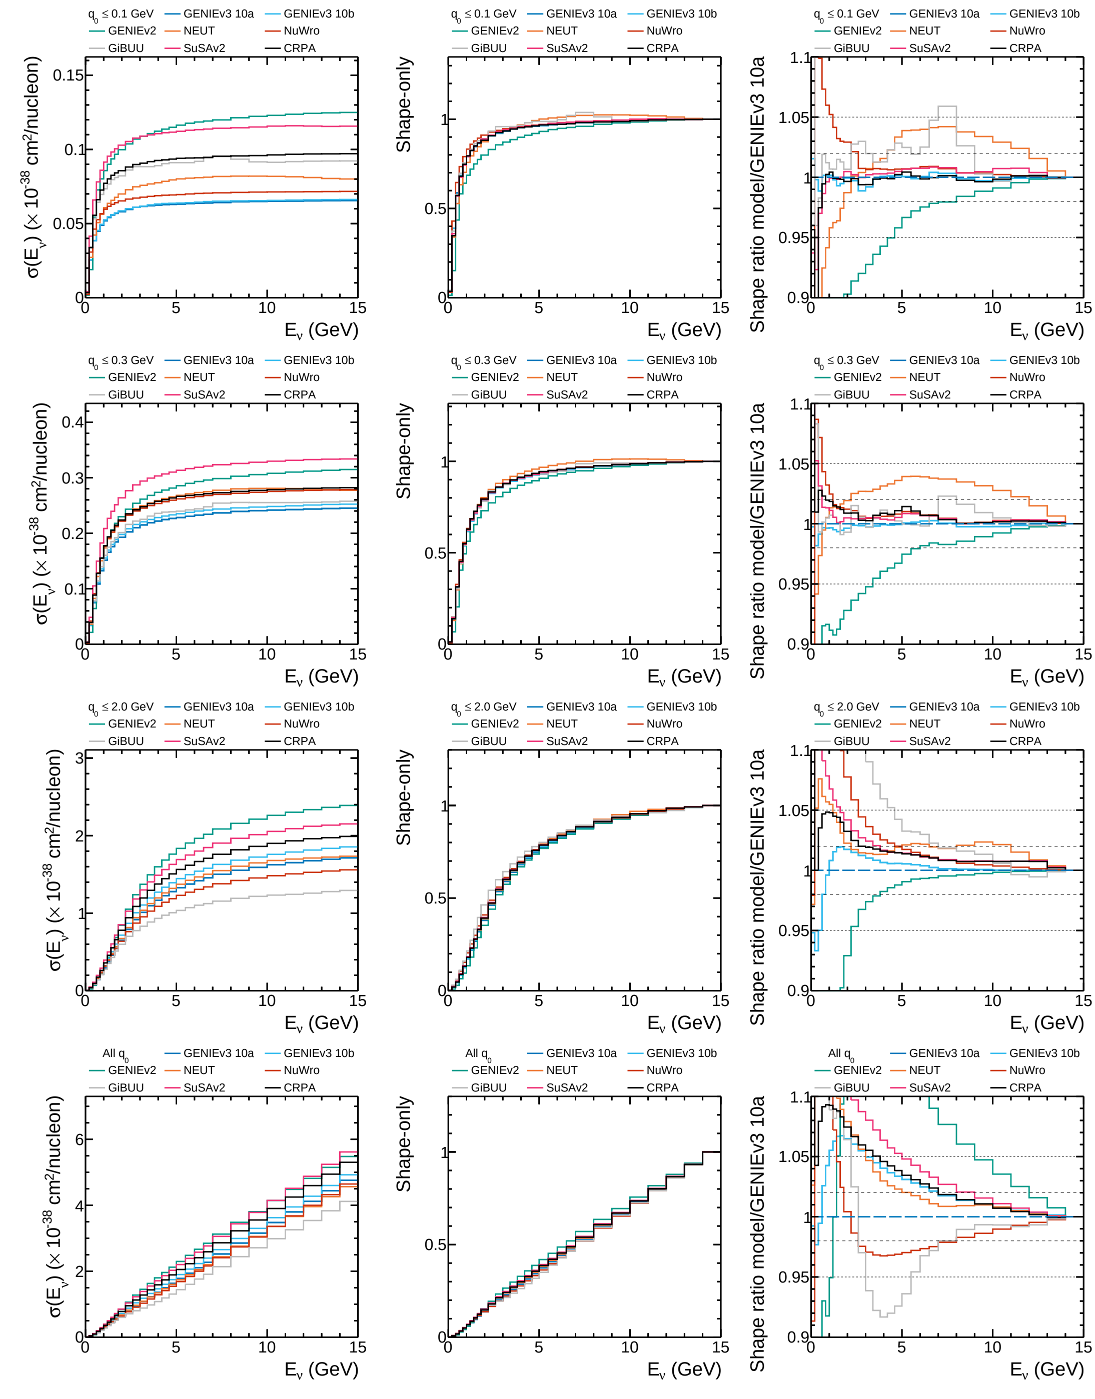


Figure 5: A comparison of the various generator predictions for different $q_0$ cuts. The absolute $\bar{\nu}_\mu$ on $C_nH_n$ cross section per nucleon (left column), a shape-only comparison where each prediction is normalized to give the same prediction for the 14–15 GeV bin (center column), and the variation of each shape-only prediction relative to a GENIEv3 10a reference prediction (right column). The four rows show the effect of increasing the $q_0$ cut 0.1 GeV, 0.3 GeV, 2.0 GeV, or having no cut, when attempting to isolate a low-$\nu$ sample.

## $\bar{\nu}_\mu$ Interacting with a $C_nH_n$ Target: Cutting on $E_{\rm had}^{\rm true}$

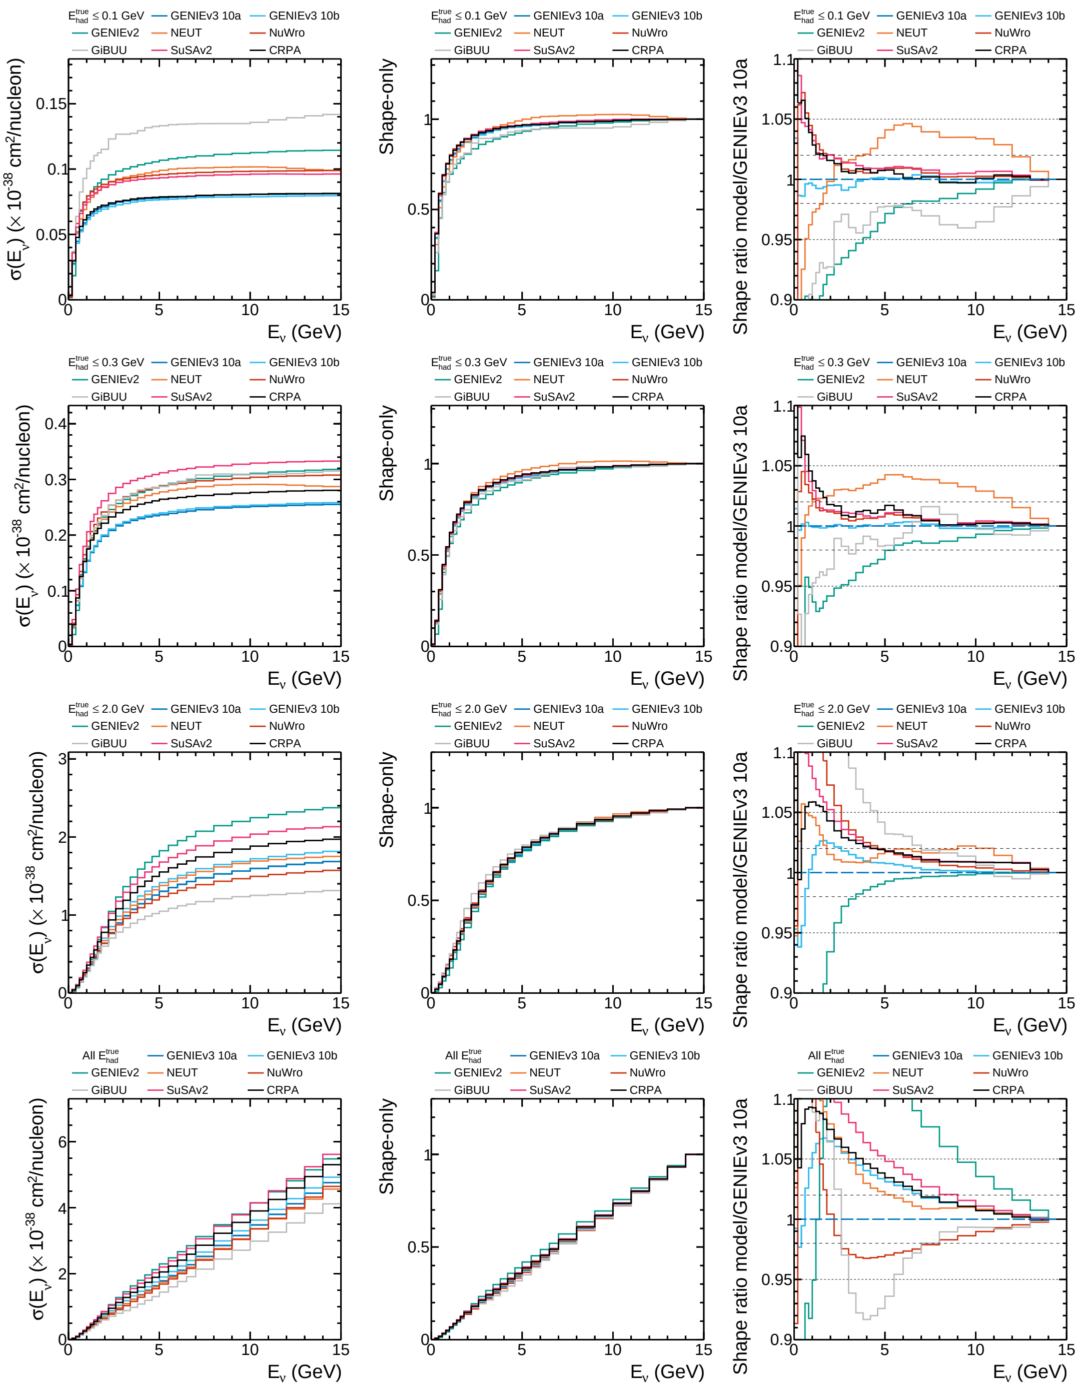


Figure 6: A comparison of the various generator predictions for different $E_{\rm had}^{\rm true}$ cuts. The absolute $\bar{\nu}_\mu$ on $C_nH_n$ cross section per nucleon (left column), a shape-only comparison where each prediction is normalized to give the same prediction for the 14–15 GeV bin (center column), and the variation of each shape-only prediction relative to a GENIEv3 10a reference prediction (right column). The four rows show the effect of increasing the $E_{\rm had}^{\rm true}$ cut 0.1 GeV, 0.3 GeV, 2.0 GeV, or having no cut, when attempting to isolate a low-$\nu$ sample.

## $\bar{\nu}_\mu$ Interacting with a $C_nH_n$ Target: Cutting on $E_{\rm had}^{\rm reco}$

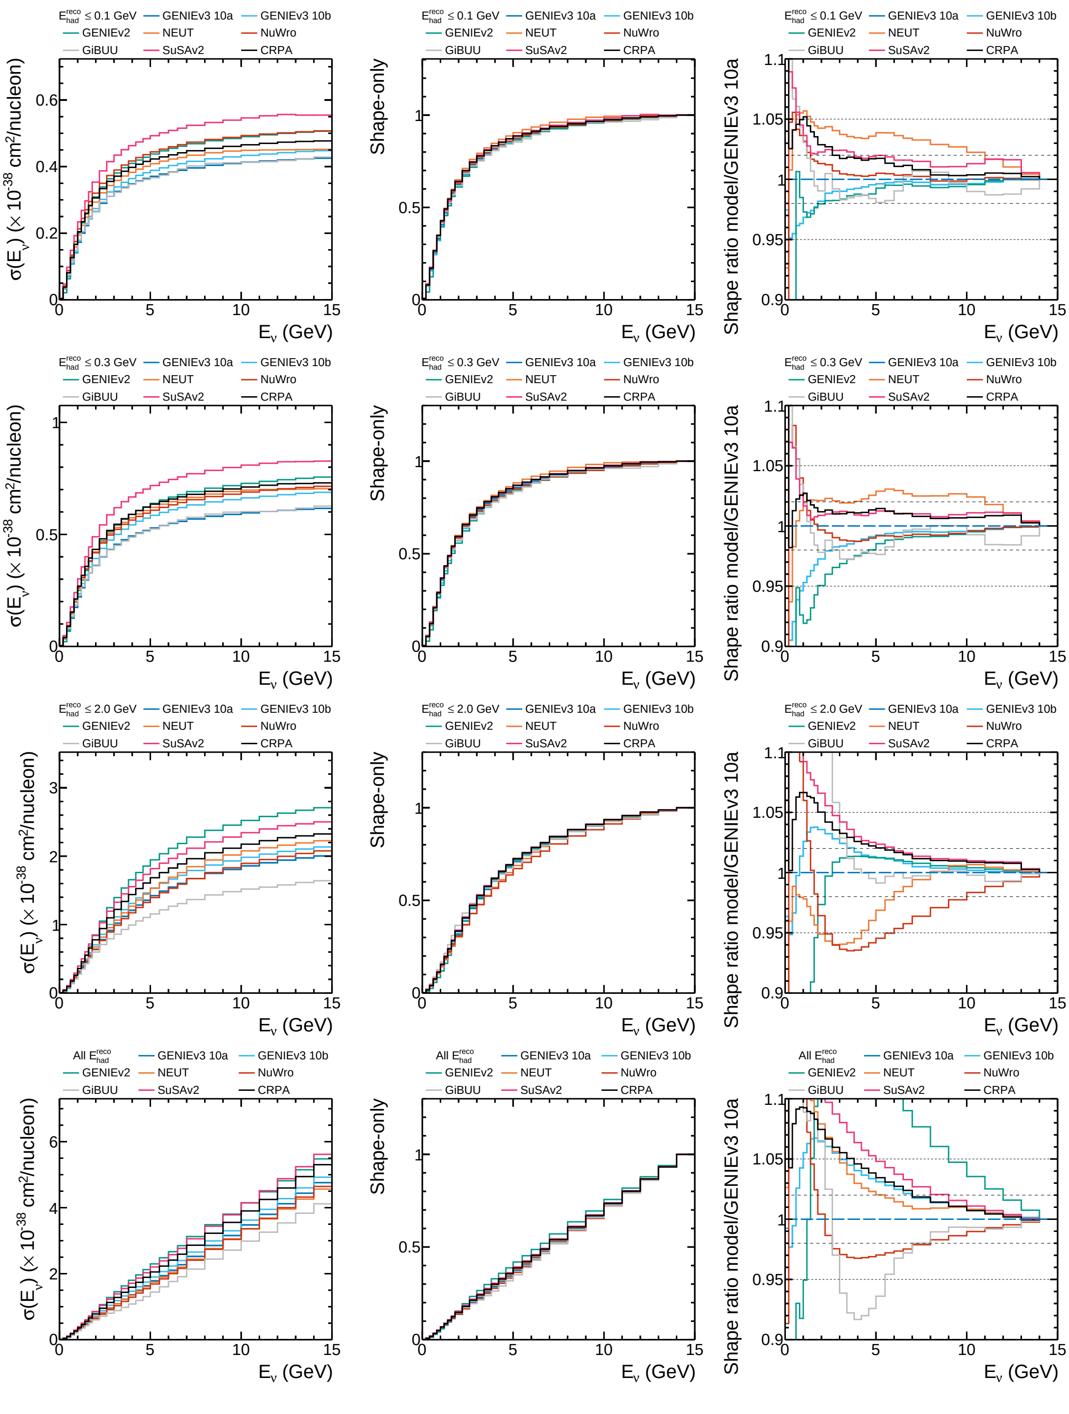


Figure 7: A comparison of the various generator predictions for different $E_{\rm had}^{\rm reco}$ cuts. The absolute $\bar{\nu}_\mu$ on $C_nH_n$ cross section per nucleon (left column), a shape-only comparison where each prediction is normalized to give the same prediction for the 14–15 GeV bin (center column), and the variation of each shape-only prediction relative to a GENIEv3 10a reference prediction (right column). The four rows show the effect of increasing the $E_{\rm had}^{\rm reco}$ cut 0.1 GeV, 0.3 GeV, 2.0 GeV, or having no cut, when attempting to isolate a low-$\nu$ sample.

## $\bar{\nu}_\mu$ Interacting with a $C_nH_n$ Target: Cutting on $E_{\mathrm{avail}}$

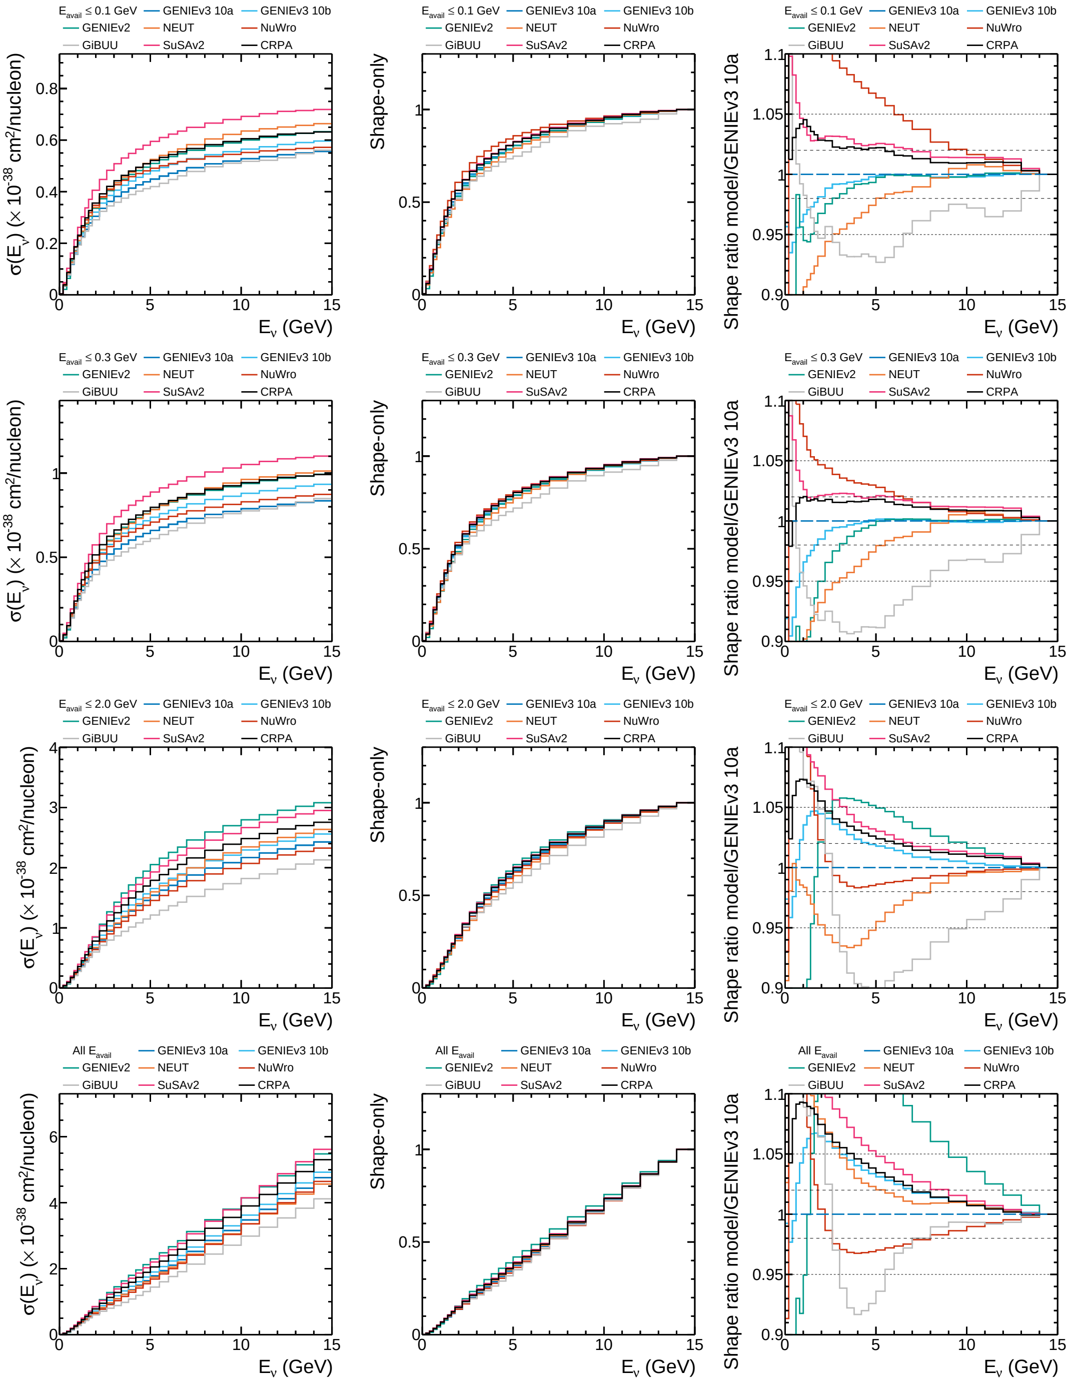


Figure 8: A comparison of the various generator predictions for different $E_{\mathrm{avail}}$ cuts. The absolute $\bar{\nu}_\mu$ on $C_nH_n$ cross section per nucleon (left column), a shape-only comparison where each prediction is normalized to give the same prediction for the 14–15 GeV bin (center column), and the variation of each shape-only prediction relative to a GENIEv3 10a reference prediction (right column). The four rows show the effect of increasing the $E_{\mathrm{avail}}$ cut 0.1 GeV, 0.3 GeV, 2.0 GeV, or having no cut, when attempting to isolate a low-$\nu$ sample.

# $\nu_\mu$ Interacting with a $^{40}$Ar Target

## $\nu_\mu$ Interacting with a $^{40}$Ar Target: Cutting on $q_0$

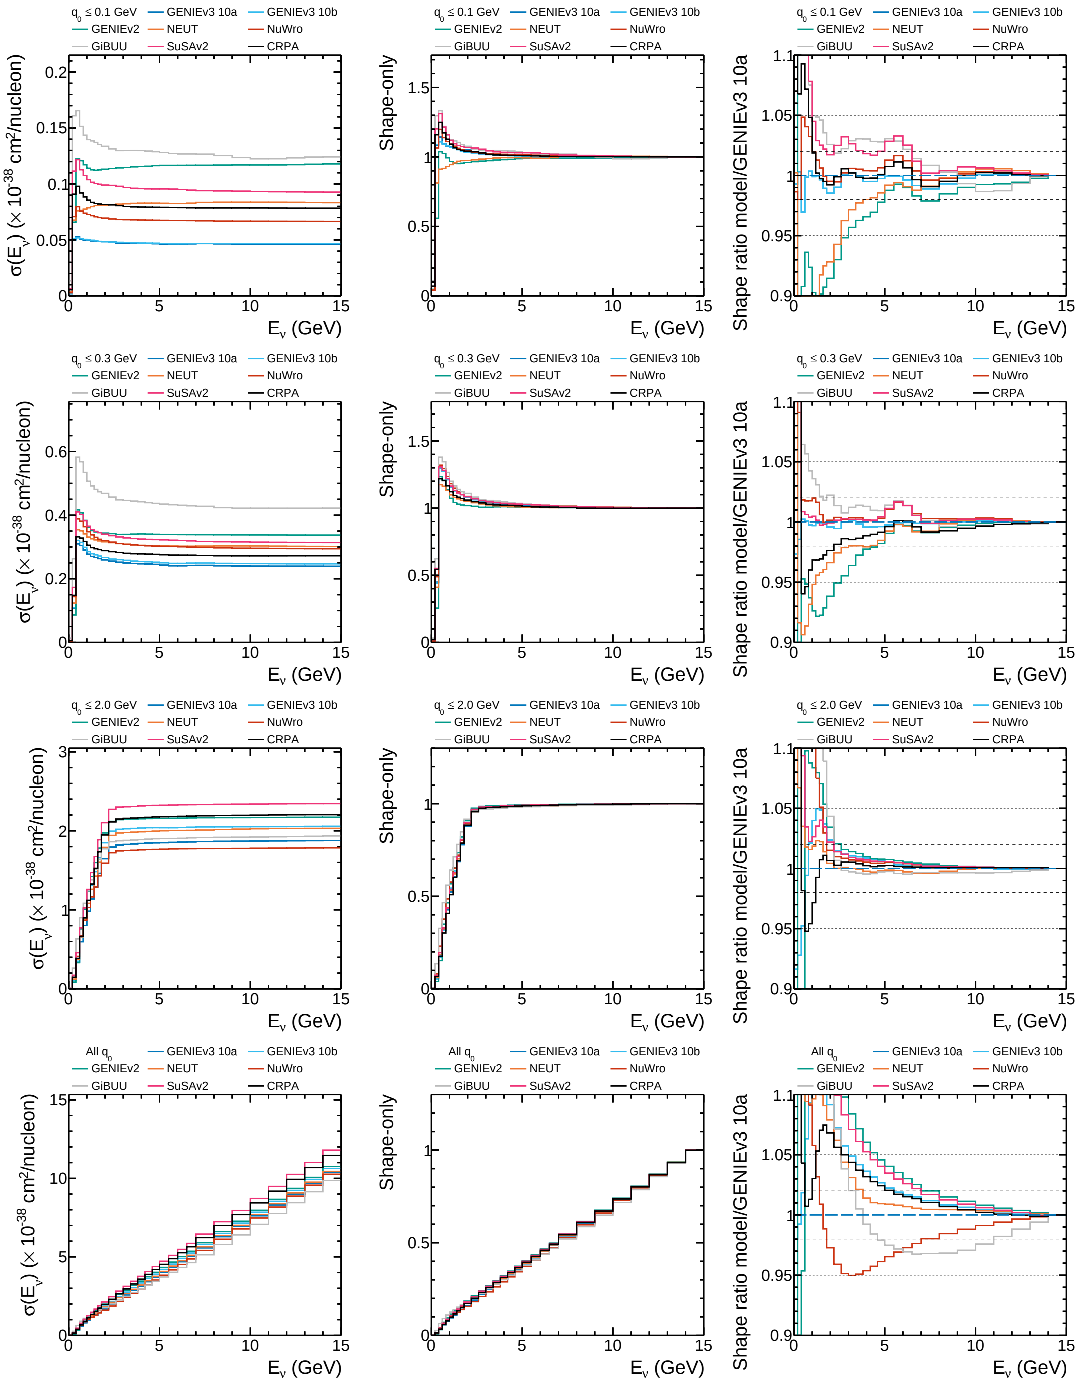

Figure 9: A comparison of the various generator predictions for different $q_0$ cuts. The absolute $\nu_\mu$ on $^{40}$Ar cross section per nucleon (left column), a shape-only comparison where each prediction is normalized to give the same prediction for the 14–15 GeV bin (center column), and the variation of each shape-only prediction relative to a GENIEv3 10a reference prediction (right column). The four rows show the effect of increasing the $q_0$ cut 0.1 GeV, 0.3 GeV, 2.0 GeV, or having no cut, when attempting to isolate a low-$\nu$ sample.

## $\nu_\mu$ Interacting with a $^{40}$Ar Target: Cutting on $E_{\rm had}^{\rm true}$

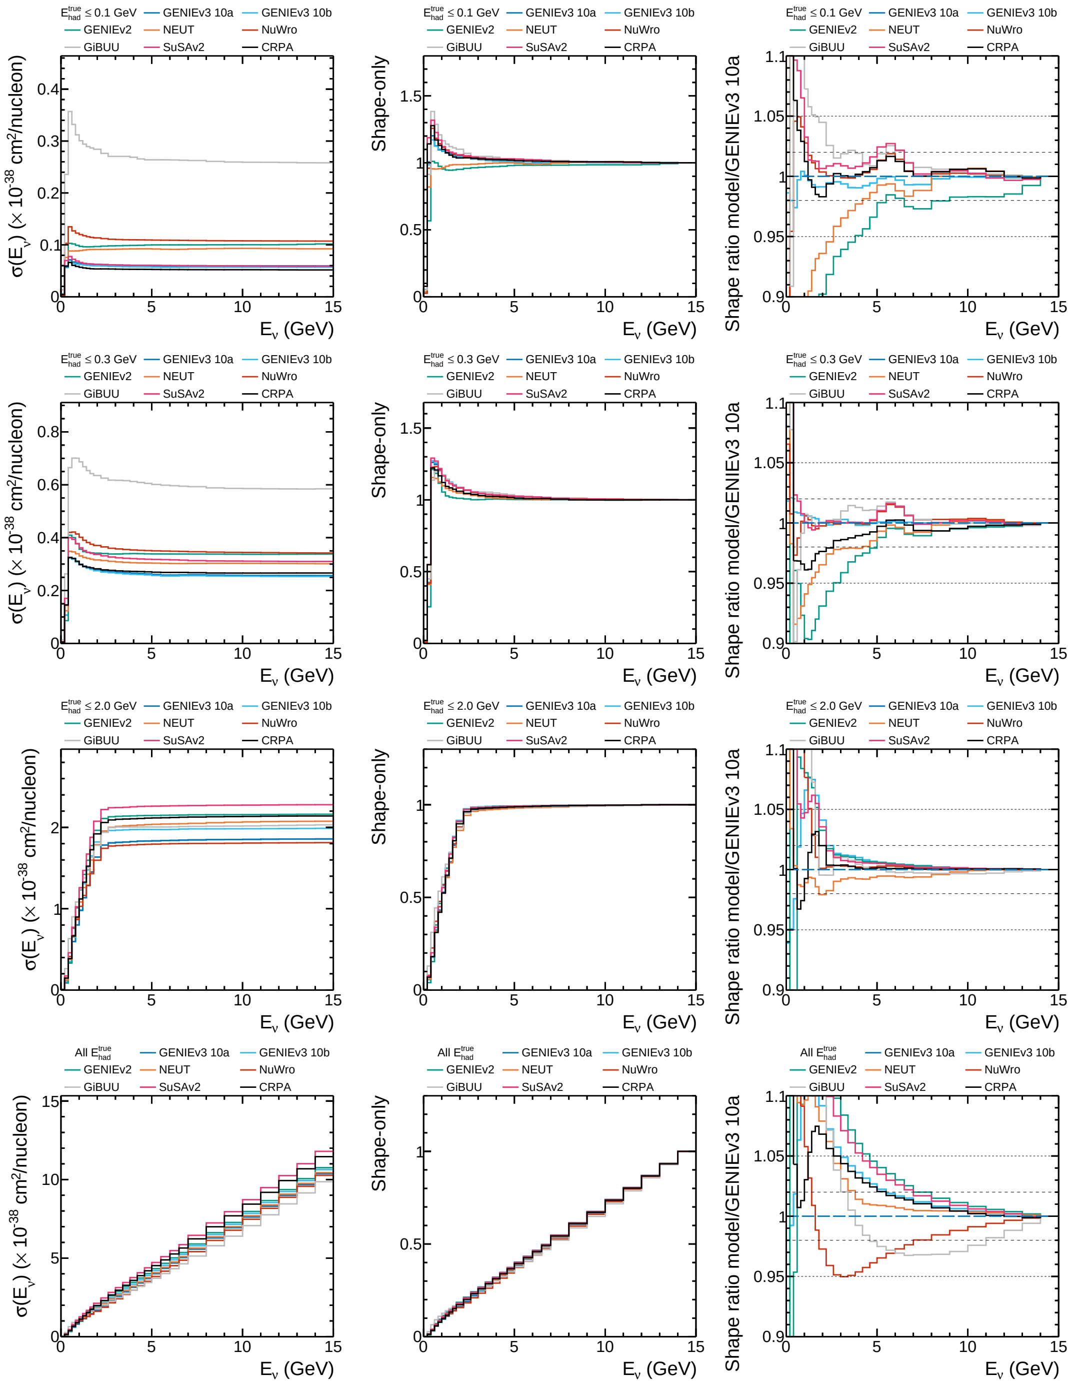


Figure 10: A comparison of the various generator predictions for different $E_{\rm had}^{\rm true}$ cuts. The absolute $\nu_\mu$ on $^{40}$Ar cross section per nucleon (left column), a shape-only comparison where each prediction is normalized to give the same prediction for the 14–15 GeV bin (center column), and the variation of each shape-only prediction relative to a GENIEv3 10a reference prediction (right column). The four rows show the effect of increasing the $E_{\rm had}^{\rm true}$ cut 0.1 GeV, 0.3 GeV, 2.0 GeV, or having no cut, when attempting to isolate a low-$\nu$ sample.

## $\nu_\mu$ Interacting with a $^{40}$Ar Target: Cutting on $E_{\rm had}^{\rm reco}$

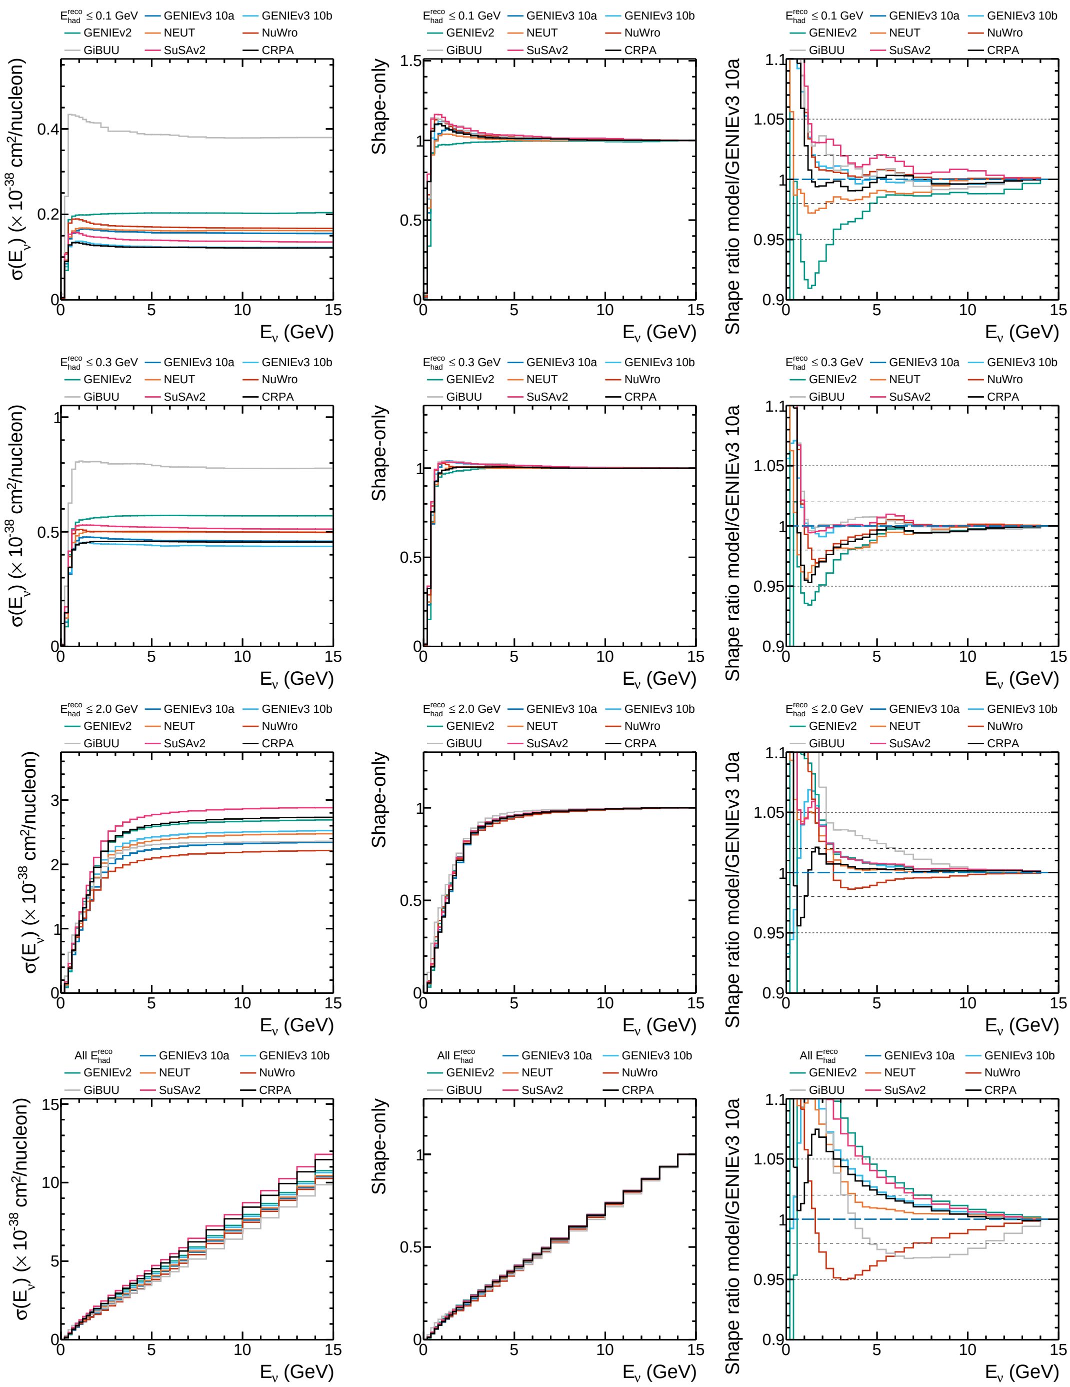


Figure 11: A comparison of the various generator predictions for different $E_{\rm had}^{\rm reco}$ cuts. The absolute $\nu_\mu$ on $^{40}$Ar cross section per nucleon (left column), a shape-only comparison where each prediction is normalized to give the same prediction for the 14–15 GeV bin (center column), and the variation of each shape-only prediction relative to a GENIEv3 10a reference prediction (right column). The four rows show the effect of increasing the $E_{\rm had}^{\rm reco}$ cut 0.1 GeV, 0.3 GeV, 2.0 GeV, or having no cut, when attempting to isolate a low-$\nu$ sample.

## $\nu_\mu$ Interacting with a $^{40}$Ar Target: Cutting on $E_{\rm avail}$

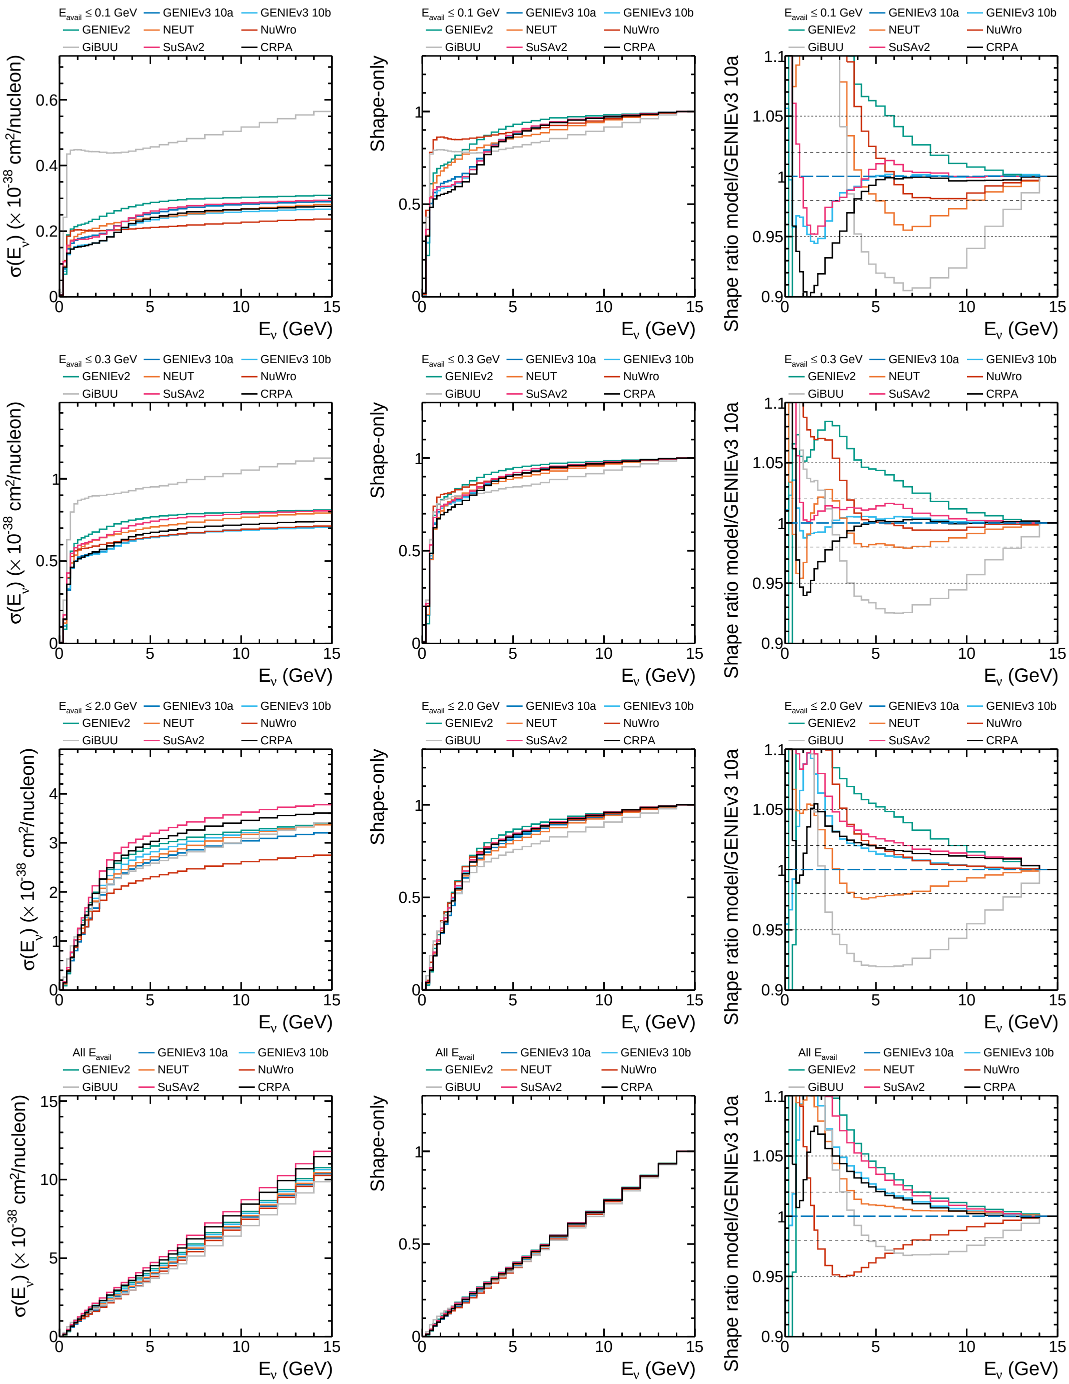


Figure 12: A comparison of the various generator predictions for different $E_{\rm avail}$ cuts. The absolute $\nu_\mu$ on $^{40}$Ar cross section per nucleon (left column), a shape-only comparison where each prediction is normalized to give the same prediction for the 14–15 GeV bin (center column), and the variation of each shape-only prediction relative to a GENIEv3 10a reference prediction (right column). The four rows show the effect of increasing the $E_{\rm avail}$ cut 0.1 GeV, 0.3 GeV, 2.0 GeV, or having no cut, when attempting to isolate a low-$\nu$ sample.

# $\bar{\nu}_\mu$ Interacting with a $^{40}$Ar Target

## $\bar{\nu}_\mu$ Interacting with a $^{40}$Ar Target: Cutting on $q_0$

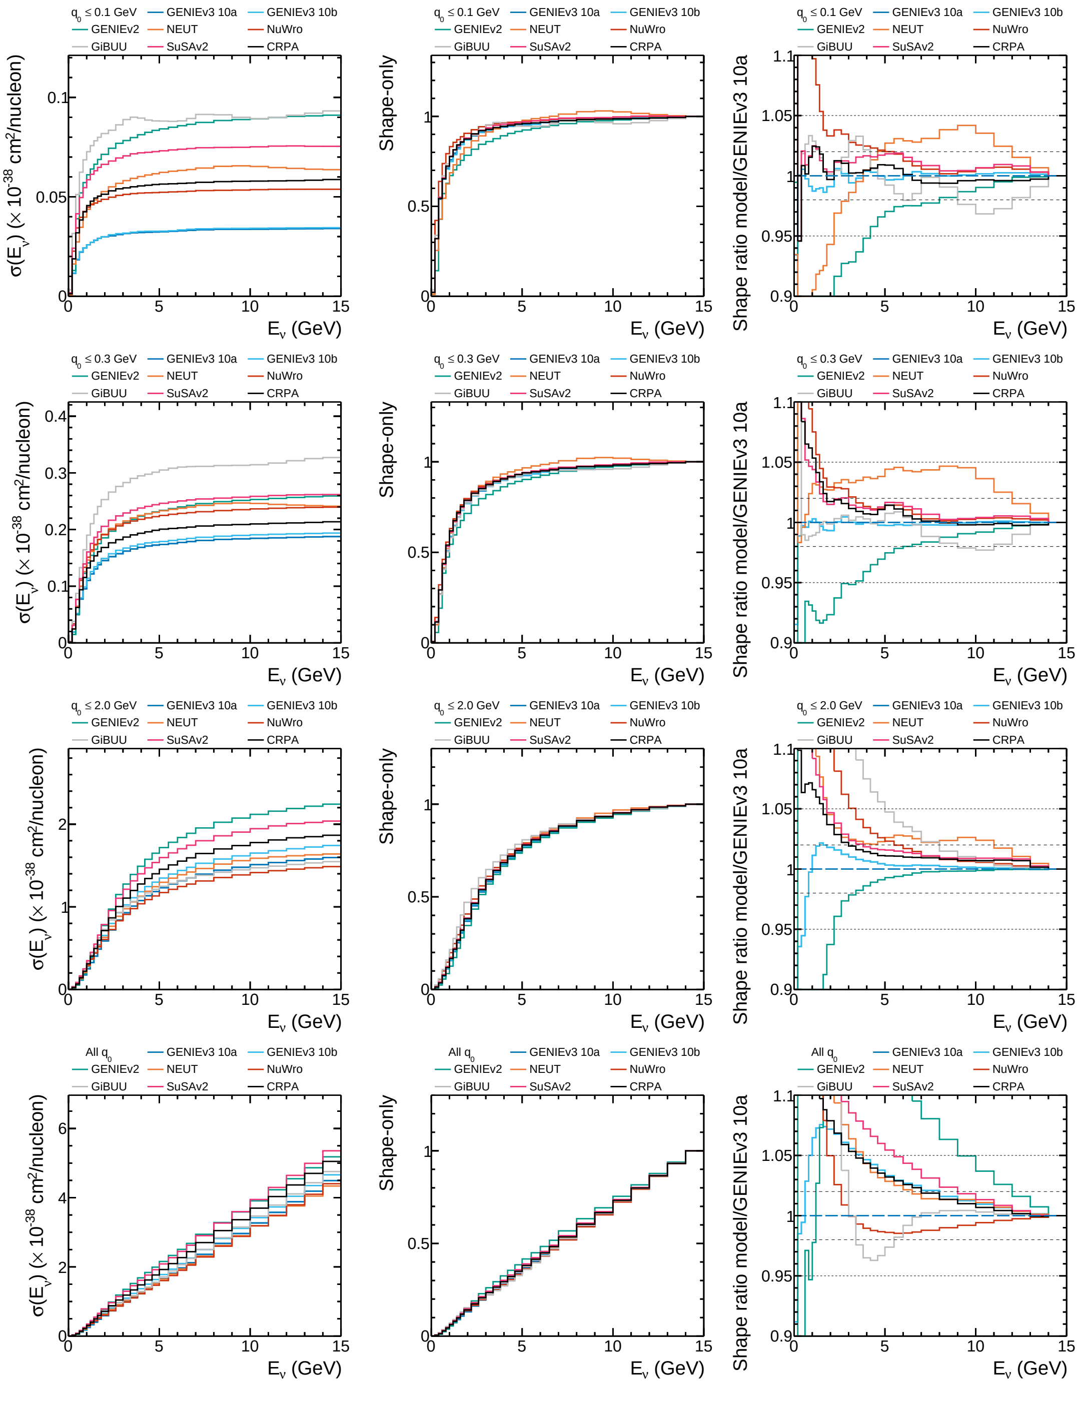


Figure 13: A comparison of the various generator predictions for different $q_0$ cuts. The absolute $\bar{\nu}_\mu$ on $^{40}$Ar cross section per nucleon (left column), a shape-only comparison where each prediction is normalized to give the same prediction for the 14–15 GeV bin (center column), and the variation of each shape-only prediction relative to a GENIEv3 10a reference prediction (right column). The four rows show the effect of increasing the $q_0$ cut 0.1 GeV, 0.3 GeV, 2.0 GeV, or having no cut, when attempting to isolate a low-$\nu$ sample.

## $\bar{\nu}_\mu$ Interacting with a $^{40}$Ar Target: Cutting on $E_{\rm had}^{\rm true}$

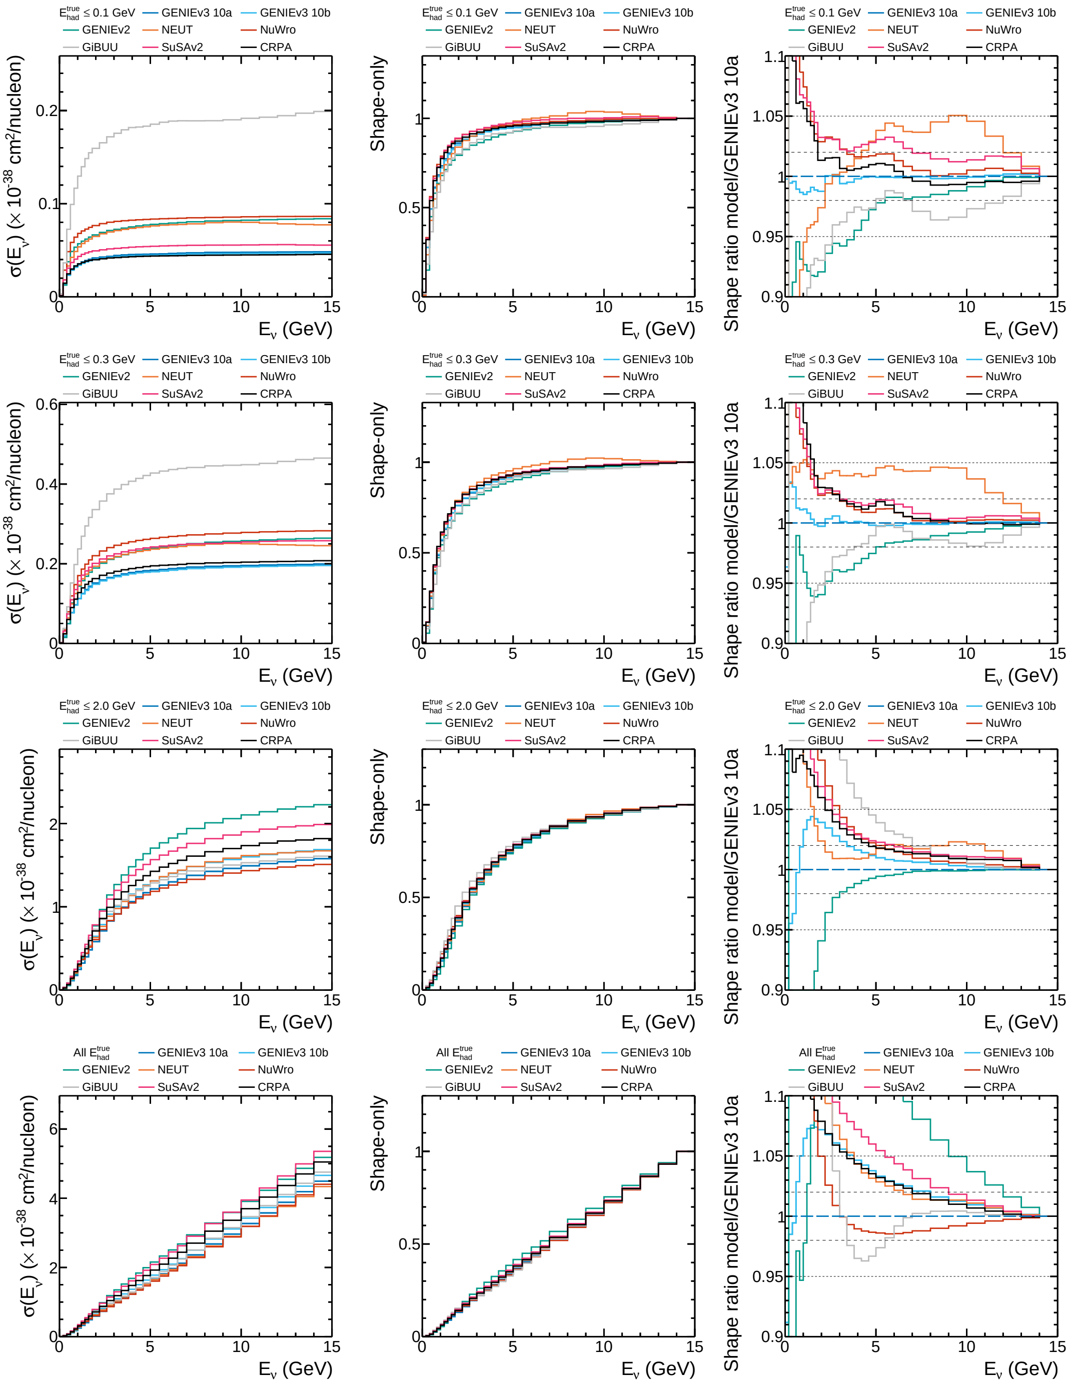

Figure 14: A comparison of the various generator predictions for different $E_{\rm had}^{\rm true}$ cuts. The absolute $\bar{\nu}_\mu$ on $^{40}$Ar cross section per nucleon (left column), a shape-only comparison where each prediction is normalized to give the same prediction for the 14–15 GeV bin (center column), and the variation of each shape-only prediction relative to a GENIEv3 10a reference prediction (right column). The four rows show the effect of increasing the $E_{\rm had}^{\rm true}$ cut 0.1 GeV, 0.3 GeV, 2.0 GeV, or having no cut, when attempting to isolate a low-$\nu$ sample.

## $\bar{\nu}_\mu$ Interacting with a $^{40}$Ar Target: Cutting on $E_{\rm had}^{\rm reco}$

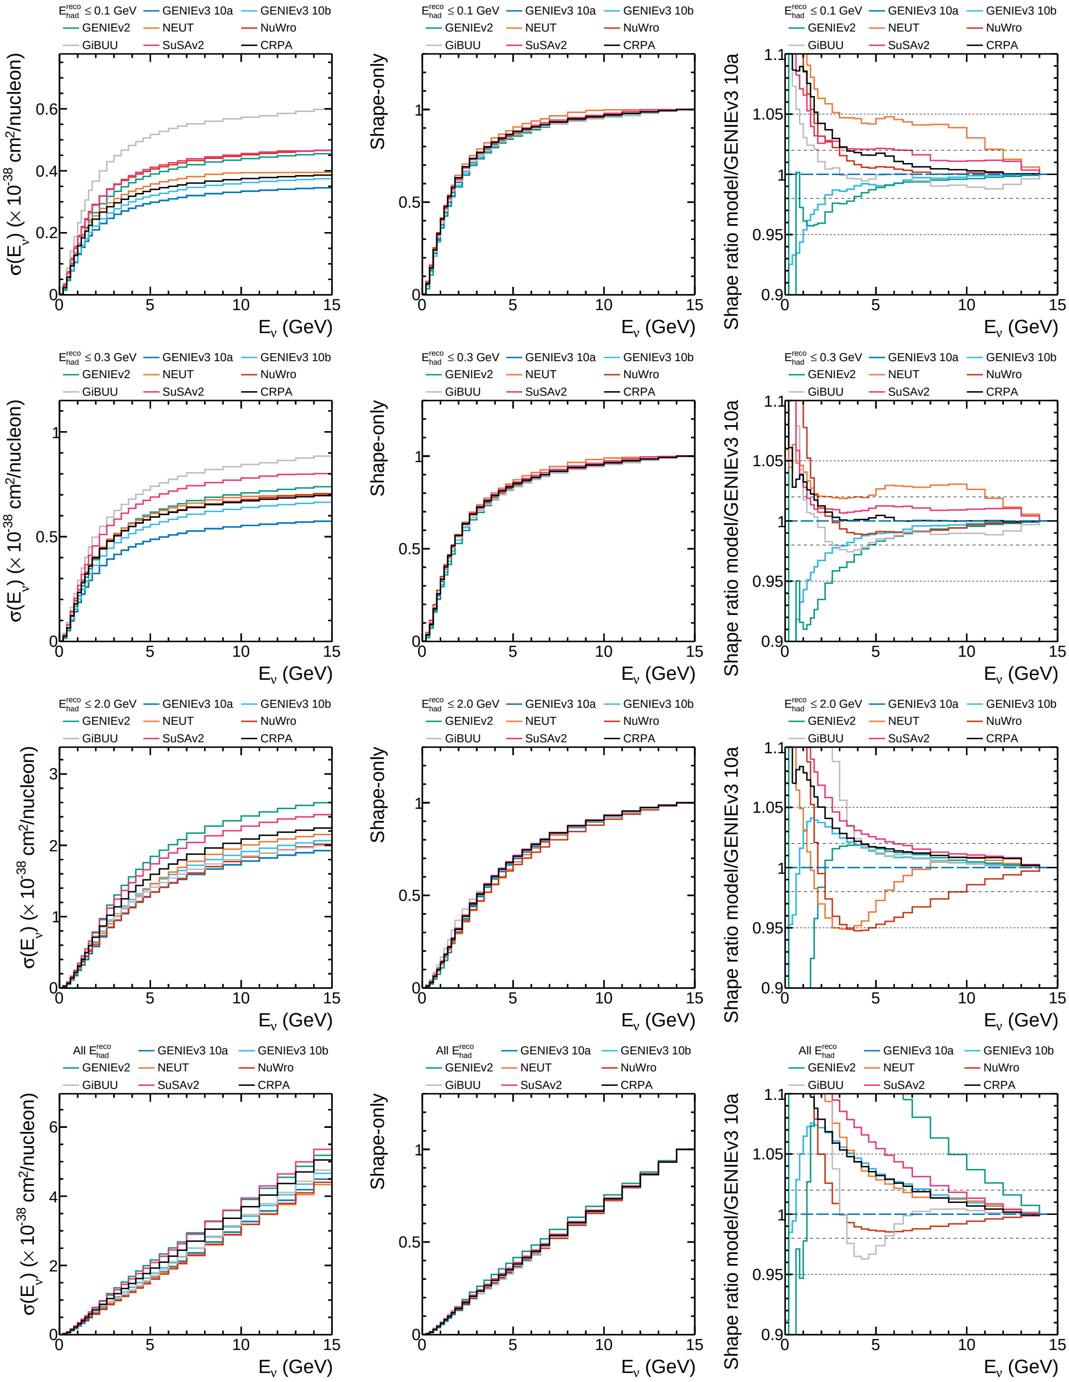


Figure 15: A comparison of the various generator predictions for different $E_{\rm had}^{\rm reco}$ cuts. The absolute $\bar{\nu}_\mu$ on $^{40}$Ar cross section per nucleon (left column), a shape-only comparison where each prediction is normalized to give the same prediction for the 14–15 GeV bin (center column), and the variation of each shape-only prediction relative to a GENIEv3 10a reference prediction (right column). The four rows show the effect of increasing the $E_{\rm had}^{\rm reco}$ cut 0.1 GeV, 0.3 GeV, 2.0 GeV, or having no cut, when attempting to isolate a low-$\nu$ sample.

## $\bar{\nu}_\mu$ Interacting with a $^{40}$Ar Target: Cutting on $E_{\text{avail}}$

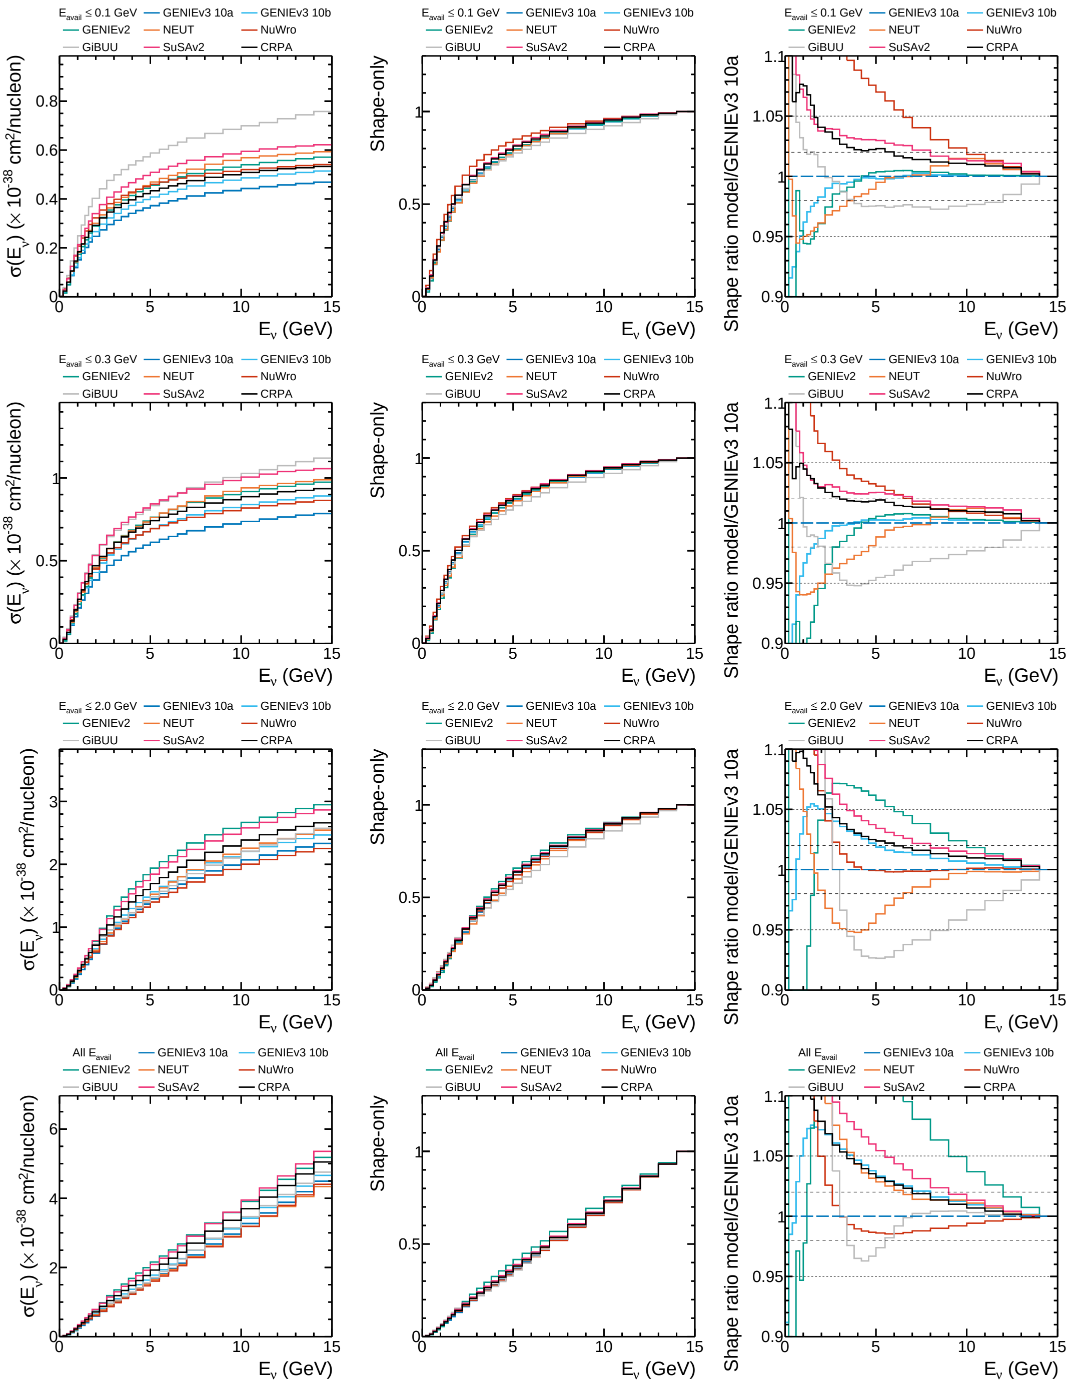


Figure 16: A comparison of the various generator predictions for different $E_{\text{avail}}$ cuts. The absolute $\bar{\nu}_\mu$ on $^{40}$Ar cross section per nucleon (left column), a shape-only comparison where each prediction is normalized to give the same prediction for the 14–15 GeV bin (center column), and the variation of each shape-only prediction relative to a GENIEv3 10a reference prediction (right column). The four rows show the effect of increasing the $E_{\text{avail}}$ cut 0.1 GeV, 0.3 GeV, 2.0 GeV, or having no cut, when attempting to isolate a low-$\nu$ sample.
